# Supplementary material for: Self-Supervised Anomaly Detection by Self-Distillation and Negative Sampling
Source: arXiv:2201.06378 source file (2022-01-17)
Supplement: Supplementary file 1 [file X_supplementary.tex]

\appendix

\setcounter{page}{1}

\twocolumn[
\centering
\Large
\textbf{Self-Supervised Anomaly Detection by Self-Distillation and Negative Sampling} \\
\vspace{0.5em}Supplementary Material \\
Paper ID 11286 \\
\vspace{1.0em}
]

\appendix
% \section{$\mathcal{D}_{train}^{in}$ and $\mathcal{D}_{test}^{out}$ dataset details}
\section{Dataset details}
For\@ self-supervised training and testing OOD performance,\@ the following datasets were considered:
\begin{itemize}
    \item  CIFAR$10$:\@ It\@ includes $50,000$ training images and $10,000$ test images from $10$ classes.
    
    \item  CIFAR$100$: It consists of $50,000$ training images and $10,000$ test images from $100$ classes.
    
    \item SVHN: It is a $10$-class dataset of digits ($0$-$9$) from real-world street view house numbers. It contains $604,388$ and $26,032$ training and test images, respectively.
    
    \item ImageNet$30$: It consists of $3,000$ test images from $30$ image classes.
    
    \item TinyImageNet:\@ TinyImageNet is a subset of ImageNet with $200$ image classes.\@ The training set has $100K$ images, while the test set has $10,000$ images. Images are resized and cropped to $64\times64$.
    
    \item LSUN:\@ It consists of $10,000$ test images of $10$ different scene categories.
    
    \item STL$10$:\@ It is an image recognition dataset inspired by the CIFAR$10$ dataset.\@ It contains $8,000$ test images.\@ Unlike the CIFAR$10$ dataset, the STL$10$ dataset has a higher resolution ($96 \times 96$).
    \item Places$365$: It consists of $1,803,460$ and $365,000$ training and test photographs of scenes, respectively.\@ Scenes are categorized into $365$ classes.
    \item Texture: The Describable Textures Dataset (DTD) is a collection of textural images in the wild.\@ It contains $5,546$ test images.
\end{itemize}
We highlight that for self-supervised training only the training images were used as $\mathcal{D}_{train}^{in}$, while at test time only the available test images were used.\@ Moreover, OOD test images and auxiliary images are resized to the in-distribution image size ($32\times32$) before applying any augmentation in all CIFAR$10$ and CIFAR$100$ experiments.

\section{Augmentation pipeline}
% To make the manuscript as self-complete as possible, the augmentation pipeline from \cite{caron2021emerging,byol}, is described.
For data augmentations $\mathcal{T}$, we adopt those used by \cite{caron2021emerging}. Additional details on the image augmentations are found in \cref{tab:transformation_distributions}.\@ $\mathcal{T}_{local}$ and $\mathcal{T}_{global}$ indicate set of augmentations used for the local and global views, respectively. Negative samples undergo the same transformations $\mathcal{T}_{local}$ and $\mathcal{T}_{global}$. If there is an additional negative transformation, it's applied before $\mathcal{T}_{global}$ and $\mathcal{T}_{local}$. Finally, all views are normalized with the ImageNet channel-wise means and variances.

\begin{table}[ht]
    \small
    \centering
    \begin{tabular}{l l l l} \toprule
        Parameters & $\mathcal{T}_{local}$ & $\mathcal{T}_{global}^{1}$&  $\mathcal{T}_{global}^{2}$ \\ \midrule
        Random crop probability & $1.0$ & $1.0$ & $1.0$\\
        Resize dimension & $128$ & $256$ & $256$ \\
        Flip probability & $0.5$ & $0.5$ & $0.5$ \\
        Color jittering probability & $0.8$ & $0.8$ & $0.8$ \\
        Brightness adjustment max intensity & $0.4$ & $0.4$ & $0.4$ \\
        Contrast adjustment max intensity & $0.4$ & $0.4$ & $0.4$ \\
        Saturation adjustment max intensity & $0.2$ & $0.2$ & $0.2$ \\
        Hue adjustment max intensity & $0.1$ & $0.1$ & $0.1$ \\
        Convert to greyscale probability & $0.2$ & $0.2$  & $0.2$  \\
        Gaussian blurring probability & $0.5$ & $1.0$ & $0.1$ \\
        Solarization probability & $0.0$ & $0.0$ & $0.2$ \\ \bottomrule
    \end{tabular}
     \vspace{0.5em}
    \caption{Parameters used to generate image augmentations of local ($\mathcal{T}_{local}$) and global views (alternating between $\mathcal{T}_{global}^1$ and $\mathcal{T}_{global}^2$).\@ Notably, auxiliary images are first resized to the size of $\mathcal{D}_{train}^{in}$ samples (e.g. $32 \times 32$ for CIFAR$10$).}
    \label{tab:transformation_distributions}
\end{table}

\begin{table*}[t]
\label{tab:contrast_dataset_cif100}
\caption{AUROC scores for OOD Detection with CIFAR$100$ as {$\mathcal{D}^{in}_{train}$} and different $\mathcal{D}_{neg}$. ImgN denotes ImageNet samples.} 
\setlength{\tabcolsep}{2pt}
\begin{center}
\begin{tabularx}{\linewidth}{c*{11}{Y}}
\hline

\multicolumn{2}{c|}{Negative Sampling:} &  \multicolumn{1}{Y|}{None} & \multicolumn{8}{c|}{Auxiliary} & \multicolumn{1}{Y}{In-Dist} \\
\hline
\parbox[t]{1.0cm}{\centering \medskip \smallskip $\mathcal{D}_{train}^{in}$}  &
\parbox[t]{1.85cm}{\centering \medskip \smallskip $\mathcal{D}_{test}^{out}$ } &  DINO  $\lambda=0$ & ImgN & Rot. ImgN & Rot.$360$ ImgN & DTI & Perm-$16$ ImgN & Perm-$4$ ImgN & \parbox[t]{1.0cm}{\centering Rot.\\DTI} & Pix. Perm. & Rot. In-Dist. \\

\hline

\multirow{11}{*}{} 
\multirow{8}{*}{\rotatebox{90}{CIFAR$100$}}

&
  \multicolumn{1}{c}{CIFAR$10$} &
                   $69.69$ & $69.29$ & $69.96$ & $70.47$ & $70.51$ & $70.37$ & $69.61$ & $69.08$ & $\mathbf{70.64}$ & $67.63$\\ % & $67.63$ \\
                   
& \multicolumn{1}{c}{SVHN} &  
                   $89.28$ & $90.30$ & $96.00$ & $95.22$ & $96.61$ & $96.39$ & $95.33$ & $97.47$ & $96.91$ & $\mathbf{97.95}$\\

& \multicolumn{1}{c}{ImageNet$30$} & 
                   $69.78$ & $71.80$ & $\mathbf{84.82}$ & $79.20$ & $76.36$ & $73.38$ & $77.00$ & $76.35$ & $74.65$ & $75.36$ \\

& \multicolumn{1}{c}{TinyImageNet} & 
                   $73.94$ & $80.25$ & $81.41$ & $80.84$ & $77.92$ & $75.26$ & $\mathbf{81.93}$ & $80.20$ & $76.28$ & $79.75$  \\           
                   
& \multicolumn{1}{c}{LSUN} & 
                   $65.43$ & $72.38$ & $\mathbf{85.03}$ & $78.01$ & $78.11$ & $70.70$ & $76.61$ & $76.99$ & $72.80$ & $74.55$  \\          

& \multicolumn{1}{c}{STL$10$} & 
                    $70.18$ & $69.14$ & $\mathbf{79.96}$ & $76.10$ & $71.58$ &  $70.49$ & $73.73$ & $69.30$ & $72.58$ & $71.70$  \\

& \multicolumn{1}{c}{Places$365$} & 
                   $67.30$ & $70.44$ & $\mathbf{81.67}$ & $77.89$ & $77.99$ & $71.43$ & $75.92$ & $75.54$ & $73.30$ & $72.79$  \\

& \multicolumn{1}{c}{Texture} & 
                   $55.73$ & $67.83$ & $\mathbf{80.65}$ & $67.76$ & $64.52$ & $61.42$ & $69.89$ & $73.36$ & $64.01$ & $77.33$  \\

\hline
& \multicolumn{1}{c}{Average} & 	
                   $69.85$ & $73.16$ & $\mathbf{82.44}$ & $78.13$ & $76.85$ &
                   $73.43$ & $77.21$ & $77.09$ & $74.95$ & $76.57$ \\
            
\hline
\end{tabularx}
%\end{adjustbox}
%} % end resize box
\end{center}
\label{tab:contrast_dataset_cif100}
\end{table*}

%  & $97.17$ \\

%  & $75.36$ \\

% TinyImageNet & 
%                    & $79.75$ \\                   
% %\multirow{10}{*}{}& 
% LSUN & 
%                   & $74.55$ \\
% %\multirow{10}{*}{}& 
% STL$10$ & 
%                   & $71.70$ \\
% %\multirow{10}{*}{}& 
% Places$365$ & 
%                   $00.00$ & $70.44$ & $\mathbf{81.67}$ & $00.00$ & $77.55$ & $71.43$ & $75.92$ & $69.37$ & $73.30$ & $71.54$ & $72.79$ \\
% Texture & 
%                   $00.00$ & $67.83$ & $\mathbf{80.65}$ & $00.00$ & $65.35$ & $61.42$ & $69.89$ & $61.497$ & $64.01$ & $77.00$ & $77.33$ \\
% %\hline
% %Average & 	
% %                   $00.00$ & $73.16$ & $\mathbf{82.38}$ & $00.00$ & $76.73$ & %$73.43$ & $77.21$ & $72.03$ & $74.95$ & $75.07$ & $76.57$ \\

\section{Additional experiments}
\subsection{Negative sampling strategies on CIFAR100}
In \cref{tab:contrast_dataset_cif100}, we study the same negative sampling strategies on CIFAR$100$ and their impact on OOD detection, as measured by AUROC ($\%$). It is observed that the highest OOD score in CIFAR$100$ is obtained without shifting high-level semantics to generate negative examples (Pix. Perm.). Moreover, Pix.\@ Perm reduces the impact of color statistics on in-distribution features, which is beneficial for detecting CIFAR$10$ as OOD due to its similar color statistics (\cref{fig:color_hist}). We also observed a significant average AUROC gain of about $9\%$ (Rot. ImgN versus ImgN) on Imagenet by adding rotations, while rotating DTI samples has no average AUROC gain. We hypothesize that a broader auxiliary dataset can be applied in a more general manner and that smaller datasets, such as DTI, contain fewer good negative samples. The optimal properties of the auxiliary dataset will be further investigated in future work.

Regarding in-distribution rotations, the performance on CIFAR$10$ is below the baseline. This result further validates that $R=\mathcal{U}(\{90^{\circ},180^{\circ},270^{\circ} \})$ is not a suitable transformation for CIFAR$100$. We qualitatively demonstrate that rotations do not always change the high-level semantics, by visualizing samples from $3$ classes of CIFAR$100$ (\cref{fig:cifar100_rot}).   

\input{fig/cifar100_rot}
\subsection{Loss balancing hyperparameter}
To study the effect of the balancing term, $\lambda$, we ran our experiments on CIFAR$10$ as $\mathcal{D}_{train}^{in}$ for different values $\lambda \in\{0.01, 0.1, 0.5, 1, 2\}$. The best results were obtained with $\lambda=1$, which was adopted for all our experiments.\@ When we combined auxiliary negative samples with in-distribution negatives we used $\lambda=0.5$ for both negative losses.

\section{Comparing color histograms for near and far OOD}
Two different datasets can share high-level semantics, such as the image categories between CIFAR$10$ and STL$10$\@ or low-level statistics. It is further investigated whether the datasets used in our study share their low-level statistics as well. As depicted in the \cref{fig:color_hist}, CIFAR$10$, CIFAR$100$ and STL$10$ have similar color histograms which provide one possible interpretation as to why detecting CIFAR$100$ from CIFAR$10$ (and vice versa) is referred to as near OOD detection \cite{contrastano_winkens}.

\input{fig/color_hist}

\begin{table*}[t]
\caption{OOD detection performance (AUROC $\%$) without label supervision,\@ $\mathcal{D}_{train}^{in}$: CIFAR$100$. Negative examples are combination of In-Dist and ImageNet samples when we take sharpening and translation as shifting transformation.}
\label{}
\setlength{\tabcolsep}{2pt}
\begin{center}
\begin{tabularx}{\linewidth}{ccccc}\\
\hline
{$\mathcal{D}_{test}^{out}$} & Rot & Rot+Sharp & Rot+Sharp+Trans & Rot+Sharp+GB \\
\hline
CIFAR$10$&$67.63$&$70.30$&$70.70$ &\\
SVHN&$97.17$&$95.91$&$95.03$ &\\
ImageNet$30$&$75.36$&$79.45$&$79.76$ &\\
TinyImageNet&$79.75$&$84.64$&$84.25$ &\\
LSUN&$74.55$&$76.17$&$76.01$ &\\
STL$10$&$71.70$&$76.19$&$79.22$ &\\
Places$365$&$72.79$&$77.47$&$77.66$ &\\
Texture&$77.33$&$78.45$&$76.40$ &\\
\hline
$10$-NN& $72.1$ & $70.19$ & $69.41$ & \\
\hline
\end{tabularx}
\end{center}
\end{table*}
